# Supplementary material for: High Resolution UDF Meshing via Iterative Networks
Source: arXiv:2509.17212 source file (2025-12-21)
Supplement: Supplementary file 1 [file supp_activation.tex]

% !TEX root = ../main.tex
% !TEX spellcheck = en-US

\begin{table}[!htb]
    
    \caption{\small \textbf{.} Median Image Consistency (IC $\uparrow$) for Cars at 512. *Resolution is halved.
    }
    % \vspace{-5mm}
    \label{tab:training_iterations}
    % \begin{scriptsize}
        % \begin{center}
            % \setlength{\tabcolsep}{3pt}
            \resizebox{\columnwidth}{!}{%
            \begin{tabular}{c|ccc} % <-- Removed two 'c' specifiers here
                Function & \multicolumn{3}{c}{1 iter.} & \multicolumn{3}{c}{2 iter.} & \multicolumn{3}{c}{5 iter.} \\
                & & First pass & Last pass & Last+1 pass & First pass & Last pass & Last+1 pass & First pass & Last pass & Last+1 pass\\
                \midrule
                % \multirow{6}{*}{512} 
                    Identity & 87.0 & 88.6 & 86.7 & 87.6 & 88.2 & 88.1 & - & - & - \\
                    Softmax & 86.5 & 87.1 & 87.3 & 87.5 & 87.8 & 87.8 & - & - & - \\
                    Sigmoid & 87.6 & 88.5 & 88.9 & - & - & - & 87.2 & 88.0 & - \\
                    Sigmoid + Random $r$ & 87.9 & 88.5 & 88.8 & - & - & - & 87.8 & 88.9 & - \\
                    \toprule
                % \multicolumn{1}{c|}{MeshUDF\cite{Guillard22b}}        &  &  &  &  \\
                % \multicolumn{1}{c|}{Ours}        &  &  & & \\
            \end{tabular}
            }
            % \vspace{-6mm}
        % \end{center}
    % \end{scriptsize}
\end{table}
